# Supplementary material for: Streaming Complexity of SVMs
Source: arXiv:2007.03633 source file (2020-07-07)
Supplement: Supplementary file 1 [file peAppendix.tex]

\section{Analysis for the Multiplicative Point Estimation Algorithm}
\label{apx:multAnalysis}

\begin{lemma}\label{lem:estimates}
Assuming Property 2, all size estimates throughout the execution of the algorithm are computed correctly within a factor of $(1\pm \eps/10)$ with high probability.
\end{lemma}
\begin{proof}
We use induction on time steps of the algorithm. As the base case, the algorithm is in the explicit regime where it is keeping all $O(\log n / \eps^3)$ first points explicitly and therefore the estimates are correct. Now suppose that the algorithm is computing the estimates correctly up to time $T$. Then at time $T$, for an interval $j_i\in \sI'$, the computed value of $\rho^*_{j_i} = \frac{C \log n}{\hat Z_{j_i} \eps^3} \geq \frac{C\log n}{(1+\eps) |Z_{j_i}|\eps^3}$, and by Property 2, we have $\rho_{j_i}\geq \rho^*_{j_i}\geq \frac{C\log n}{(1+\eps) |Z_{j_i}|\eps^3}$. The expectation of our estimate at time $T$ is,
$$ \mathbb{E}[\hat Z_{j_i}^T] = \mathbb{E}[ |\sE_{j_i}| / \rho_{j_i}] = \frac{1}{\rho_{j_i}}\sum_{p\in Z_{j_i}} {\textbf{1}}[p\mbox{ is sampled}]= \frac{1}{\rho_{j_i}}\sum_{p\in Z_{j_i}} \rho_{j_i} = |Z_{j_i}^T|.$$
Applying Chernoff, we get that it also holds with high probability that $\hat Z_{j_i}\approx |Z_j|$:
$$\mathbb{P}[|\hat Z_{j_i} - |Z_{j_i}| |\geq (\eps/10)|Z_{j_i}| ] \leq \exp(- \frac{\eps^2 |Z_{j_i}| \rho_{j_i}}{3}) \leq \exp(\frac{C\log n}{3(1+\eps)\eps}) \leq 1/n^3$$
for $\eps\leq 1$ and large enough $C$. Using a union bound over all $n$ time steps of the algorithm and all $m$ intervals, we get that the estimates are correct at all times of the execution of the algorithm with high probability.
\end{proof}

\begin{lemma}\label{lem:split-ratio}
At the split stage of the algorithm, using the sample set $\sE_{j_{i+1}}$ the index $\ell$ can be found successfully with high probability. That is, we can choose $\ell\in \sE_{j_{i+1}}$ such that $(1+2\eps) \leq \frac{\hat Z_{\ell}}{\hat Z_{j_i}} \leq (1+3\eps)$ and $(1+2\eps) \leq \frac{\hat Z_{j_{i+1}}}{\hat Z_{\ell}} \leq (1+3\eps)$.
\end{lemma}
\begin{proof}
Note that when we split, we have that $\frac{\hat Z_{j_{i+1}}}{\hat Z_{j_i}}\geq (1+6\eps)$. So let $A = \sE_{j_{i+1}}\setminus Z_{j_i}$ be all samples that are between $x_{j_i}$ and $x_{j_{i+1}}$. The size of this sample is more than $(C/2)\eps^2 \log n$ with high probability. Let $\ell$ be the $\ceil {|A|\cdot (2.5/6)}$. Then with high probability,  $(1+2\eps) \leq \frac{\hat Z_{\ell}}{\hat Z_{j_i}} \leq (1+3\eps)$, and $(1+2\eps) \leq \frac{\hat Z_{j_{i+1}}}{\hat Z_{\ell}} \leq (1+3\eps)$.
\end{proof}

\begin{definition}
For $k\leq m$, call the interval $Z_k$ \emph{unsaturated} if $\frac{\hat{Z}_{j_k}}{\hat{Z}_{j_{k-1}}}<(1+\eps)$. We call it \emph{saturated} otherwise.
\end{definition}

\begin{observation}[Property 1]\label{obs:half-saturated}
At any time step of the algorithm, for $k\leq m$, if the interval $Z_{j_k}$ is saturated, then we have $(1+\eps) \leq \frac{\hat Z_{j_k}}{\hat Z_{j_{k-1}}}<(1+6\eps)$. Moreover, at most half of the intervals are unsaturated.
\end{observation}
\begin{proof}
%Note that when we add a point $x$ that is between $x_{j_i} \leq x \leq x_{j_{i+1}}$, we can only increase the ratio of $\frac{|Z_{j_{i+1}}|}{|Z_{j_i}|}$ (for $k>i$, the value $\frac{|Z_{j_{k+1}}|}{|Z_{j_k}|}$ can only decrease, and for $k<i$, the value $\frac{|Z_{j_{k+1}}|}{|Z_{j_k}|}$ does not change). Therefore, we always maintain the property that $\hat Z_{j_{i+1}} / \hat Z_{j_i} \leq (1+6\eps)$. This means that 
%$$\frac{|Z_{j_{i+1}}|}{|Z_{j_i}|} \leq \frac{\hat Z_{j_{i+1}} (1+\eps)}{\hat Z_{j_i} (1-\eps)} \leq \frac{(1+6\eps)(1+\eps)}{(1-\eps)} \leq (1+9\eps)$$
%for small enough $\eps$.
%Also, for an interval that is saturated, we have that 
%$$\frac{|Z_{j_{i+1}}|}{|Z_{j_i}|} \geq \frac{\hat Z_{j_{i+1}} (1-\eps)}{\hat Z_{j_i} (1+\eps)} \geq \frac{(1+4\eps)(1-\eps)}{(1+\eps)} \geq (1+\eps)$$
%for small enough $\eps$.
Note that by the description of the algorithm, we always maintain the ratio property for saturated intervals.
Moreover, whenever there appears an unsaturated interval, if its previous interval is also unsaturated, we merge the two. Therefore, at least half of the intervals are saturated.
\end{proof}

\begin{corollary}\label{cor:interval-count}
The total number of indices in $\sI'$ is $O(\log n / \eps)$.
\end{corollary}
\begin{proof}
Since by Observation \ref{obs:half-saturated} at least half of the intervals are saturated, the total number of intervals is bounded by $2 \log_{1+\eps} n \leq O((\log n)/\eps)$.
\end{proof}

\begin{lemma}\label{lem:start-high}
Let $k < m$ and take $j_k$ and $j_{k+1}$ as two consecutive indices in $\sI'$ at any time step of the algorithm. Then the moment $T$ when $j_k$ and $j_{k+1}$ have become adjacent in $\sI'$,  their ratio is at least $\frac {\hat{Z}_{j_{k+1}}^T}{\hat{Z}_{j_k}^T}\geq 1+2\eps$.
\end{lemma}
\begin{proof}
At the moment when $j_k$ and $j_{k+1}$ have become adjacent, there are three possibilities.
\begin{itemize}
\item Index $j_{k}$ is added to $\sI'$ via a split operation. In this case by Lemma \ref{lem:split-ratio}, we know that $\frac {\hat{Z}_{j_{k+1}}^T}{\hat{Z}_{j_k}^T}\geq 1+2\eps$.
\item Index $j_{k+1}$ is added to $\sI'$ via a split operation. Again, by Lemma \ref{lem:split-ratio}, we know that $\frac {\hat{Z}_{j_{k+1}}^T}{\hat{Z}_{j_k}^T}\geq 1+2\eps$.
\item An index (call it $\ell$) is removed from $\sI'$ between $j_k$ and $j_{k+1}$ due to a merge operation. There could be two cases. (i) Before the merge $\frac{\hat Z_{j_{k+1}}}{\hat Z_{\ell}} \geq (1+\eps)$ and $\frac{\hat Z_{\ell}}{\hat Z_{j_k}} \geq (1+\eps)$. In this case, $\frac {\hat{Z}_{j_{k+1}}^T}{\hat{Z}_{j_k}^T}\geq 1+2\eps$. (ii) Before the merge  $\frac{\hat Z_{j_{k+1}}}{\hat Z_{\ell}} < (1+\eps)$ and $\frac{\hat Z_{\ell}}{\hat Z_{j_k}} > (1+4\eps)$. In this case $\frac {\hat{Z}_{j_{k+1}}^T}{\hat{Z}_{j_k}^T}\geq (1+4\eps)\frac{1-\frac{\eps}{10}}{1+\frac{\eps}{10}}\geq 1+2\eps$.\qedhere
\end{itemize}
\end{proof}

\begin{lemma}\label{lem:decreasing-prop}
$\rho_{j_i}^*$ is always ``almost'' non-increasing except when we merge and remove $j_{i-1}$ from $\sI'$; i.e., for any $T'>T$, unless $j_{i-1}$ is removed from $\sI'$ due to a merge operation, $\rho^{T'}_{j_i} \leq (1+\eps) \rho^T_{j_i}$.
\end{lemma}
\begin{proof}
Note that the ``almost" non-increasing (rather than non-increasing) property is due to the estimation error of $\hat{Z}$. In other words, if instead we could use the actual $|Z|$ values in the definition of $\rho^*$, the values of $\rho^*_{j_i}$ would be non-increasing. In the rest of the proof, we ignore the estimation error due to $\hat{Z}$ and show that $\rho^*_{j_i}$ is a non-increasing sequence over time if no merge operation is performed on $j_{i-1}$. Consider the following cases:
\begin{itemize}
\item{The new item in the stream is added to $Z_{j_i}$ but does not result in a split operation. As in this case the size of $Z_{j_i}$ increases, $\rho^*_{j_i}$ decreases.}
\item{The new item in the stream is added to $Z_{j_i}$ and results in a split operation. After a split operation in the interval $Z_{j_i}$, $\rho^*_{j_i}$ is multiplied by $|Z_{j_{i-1}}| / |Z_\ell| \leq 1$ where $\ell$ is the newly added index between $j_{i-1}$ and $j_i$.} \qedhere
\end{itemize} 
\end{proof}

\begin{lemma}[Property 2]\label{lem:prop2}
Property 2 always holds for any $j_i\in \sI'$.
\end{lemma}
\begin{proof}
The property that $\rho_{j_i}$ never increases trivially holds by description of the algorithm. Moreover, in the algorithm whenever we change $\rho^*_{j_i}$ or $\rho_{j_i}$, we always cap $\rho_{j_i}$ at $2 \rho^*_{j_i}$. So it remains to show that we always have $\rho^*_{j_i}\leq \rho_{j_i}$. Note that by Lemma \ref{lem:decreasing-prop}, $\rho^*$ is always almost non-increasing except on a merge operation. So we only need to show that after a merge operation we still have $\rho^*_{j_i}\leq \rho_{j_i}$. Here we use a charging argument, and on a high level, we show that before a merge operation, $\rho_{j_i}$ always hits its cap, i.e., $\rho_{j_i} = 2\rho^*_{j_i}$. Therefore, since after a merge operation the value of $\rho^*_{j_i}$ decreases by only a factor of $(1+\Theta(\eps))$, then we still have that $\rho^*_{j_i}\leq \rho_{j_i}$.

Consider the moment $T$ when the merge operation happens and we want to remove the index $j_i$. Then consider the last time $T'$ that $j_i$ and $j_{i+1}$ became adjacent in $\sI'$. By Lemma \ref{lem:start-high}, $\hat Z_{j_{i+1}}^{T'} / \hat Z_{j_i}^{T'} \geq (1+2\eps)$. Also we know that at the current time $T$, we have $\hat Z_{j_{i+1}}^{T} / \hat Z_{j_i}^{T} \leq (1+\eps)$. Therefore, $\hat{Z}^T_{j_i} \geq 2\hat{Z}^{T'}_{j_i}$ which implies that the value of $\rho^*_{j_i}$ has decreased by a factor of at least $2$ from time $T'$ to time $T$. Since by induction $\rho^{T'}_{j_i} \geq (\rho^*_{j_i})^{T'}$ and $\rho_{j_i}$ does not decrease unless it hits the cap of $\rho_{j_i} = 2\rho^*_{j_i}$, either $\rho^{T}_{j_i} = \rho^{T'}_{j_i}$ or $\rho^{T''}_{j_i} = 2(\rho^{*}_{j_i})^{T''}$ for a $T'< T'' < T$. In the former case, since $(\rho^*_{j_i})^T \leq (\rho^*_{j_i})^{T'} /2$, $\rho^{T}_{j_i} = 2(\rho^*_{j_i})^T$. In the latter case, since $\rho^{T''}_{j_1} = 2(\rho^{*}_{j_i})^{T''}$ and $\rho^*_{j_i}$ is non-increasing, $\rho^{T}_{j_i} = 2(\rho^*_{j_i})^T$. 
\end{proof}
\begin{theorem}\label{thm-pe-mult-main}
There exists a 1-pass streaming algorithm that achieves a $(1+\eps)$ multiplicative approximation for the point estimation variant of the problem that works with high probability and uses space of $O(\log^2 n / \eps^4)$.
\end{theorem}
\begin{proof}
Lemma \ref{lem:prop2} shows that Property 2 holds, and therefore using Lemma \ref{lem:estimates} we know that all estimates are correct up to a factor of $(1+\eps/10)$. Therefore, by Observation \ref{obs:half-saturated}, Property 1 also holds for the actual ratios of $|Z_{j_i}|$ upto an additional factor of $(1\pm\eps/10)$.
Now given Property 1, we can use the same algorithm as the sketching variant for processing a query.

\medskip
It only remains to show that similar to the sketching algorithm, for any $i\leq m$, we can also approximately compute the values $S_{j_i} = \sum_{k\in Z_{j_i}\setminus Z_{j_{i-1}}} (x_{j_i}-x_k)$.
Define $Y_{j_i} = Z_{j_i}\setminus Z_{j_{i-1}}$, and suppose all distances between the query point and the points in $Y_{j_i}$ are between $\delta_i$ and $\delta_{i-1}$, where $\delta_{i-1}\geq \delta_{i}$. Since we maintain $\Theta(\log n / \eps^3)$ samples from $Z_{j_i}$ in $\sE_{j_i}$, and $|Y_{j_i}| = \Theta(\eps\cdot|Z_{j_i}|)$, then with high probability, we have $\Theta(\log n /\eps^2)$ samples from $Y_{j_i}$. Therefore, we can compute a $(1+\eps)$ approximation of $|Y_{j_i}|$ by our sample set in this interval. Further, using this estimate, and employing Hoeffding bound (again using the $\Theta(\log n / \eps^2)$ samples in $Y_{j_i}$), we can also estimate $S_{j_i}$ up to an additive error of $O(\delta_{i-1}\cdot \eps|Y_{j_i}|)$. Now, since $|Y_{j_i}| \leq 2 |Y_{j-1}|$ and the minimum distance of any point in $Y_{j_{i-1}}$ from the query point is at least $\delta_{i-1}$, this additive error translates into a multiplicative error in terms of $S_{j_{i-1}}$. Thus, we can charge this estimation error for the total distance of the points in $Y_{j_i}$ from the query, to the value of $S_{j_{i-1}}$. Furthermore, note that we are explicitly maintaining the first few intervals, namely, all the first $\Theta(\log n / \eps^3)$ points, and therefore, there is no error for $S_{j_i}$ for small value of $i$. Hence this charging argument is correctly computing a $(1+\eps)$ approximation of $\sum_{i\leq r} S_{j_i}$, for any $r\leq m$, as is required by the sketching algorithm. We remark that in the sketching algorithm we use the largest value $r$ such that $x_{j_r}\leq q$.
\medskip

The rest of the proof follows similarly as the sketching variant.
Further, by Corollary \ref{cor:interval-count}, the total number of intervals is $O(\log n /\eps)$ and for each interval we maintain a sample of size $O(\log n /\eps^3)$, showing the space bound.
\end{proof}
